# Supplementary material for: Multiple Waves Propagate in Random Particulate Materials
Source: arXiv:1810.10816 ancillary file (2019-08-11)
Supplement: Supplementary file 1 [file supplement_multiple.pdf]

# SUPPLEMENTARY MATERIALS: MULTIPLE WAVES PROPAGATE IN RANDOM PARTICULATE MATERIALS*

ARTUR L. GOWER‡†, WILLIAM J. PARNELL‡, AND I. DAVID ABRAHAMS§

**Abstract.** Here we present details on: deducing the dispersion equation (3.9) and extinction theorem (3.10) in Section SM1, we deduce complex least squares with a constraint in Section SM2, which is needed for the matching method. To help understand and implement the matching method we provide Algorithm SM3.1 in Section SM3 .

**SM1. Equations for effective waves.** Here we show how substituting the effective wave series (3.8) into the governing equation (2.20) leads to the equations (3.10) and (3.9). Many of the details here can be found in [SM2, SM1].

$$\mathcal{A}_n(X) = \mathrm{i}^n \sum_{p=1}^{P} \mathrm{e}^{-\mathrm{i}n\varphi_p} A_n^p \mathrm{e}^{\mathrm{i}XK_p\cos\varphi_p} \quad \text{for} \quad X > \bar{X}, \tag{SM1.1}$$

Substituting the sum of plane waves above into the system (2.20), and assuming $kx_1 > \bar{X} + ka_{12}$, leads to the integral

$$\int_{\substack{x_2>0 \\ \|\mathbf{x}_1-\mathbf{x}_2\|>a_{12}}} \mathcal{A}_n(kx_2)\mathrm{e}^{\mathrm{i}k(y_2-y_1)\sin\theta_{\mathrm{inc}}} F_{n-m}(k\mathbf{x}_2 - k\mathbf{x}_1)d\mathbf{x}_2 = \tag{SM1.2}$$
$$\frac{\mathrm{i}^n}{k^2}\sum_{p=1}^{P} \mathrm{e}^{-\mathrm{i}n\varphi_p} A_n^p \mathrm{e}^{\mathrm{i}X_1K_p\cos\varphi_p} \int_{\substack{X>\bar{X}-X_1 \\ \|\mathbf{X}\|>\gamma R_o}} \mathrm{e}^{\mathrm{i}XK_p\cos\varphi_p}\mathrm{e}^{\mathrm{i}Y\sin\theta_{\mathrm{inc}}} F_{n-m}(\mathbf{X})d\mathbf{X}$$
$$+ \frac{1}{k^2}\int_0^{\bar{X}} \mathcal{A}_n(X_2)L_{n-m}(X_2 - X_1)dX_2$$

where $Y = k(y_2 - y_1)$, $X = k(x_2 - x_1)$, and

$$L_{n-m}(X) = \int_{-\infty}^{\infty} \mathrm{e}^{\mathrm{i}Y\sin\theta_{\mathrm{inc}}} F_{n-m}(\mathbf{X})dY. \tag{SM1.3}$$

From [SM3, Eq. (37)] we have

$$L_n(X) = \begin{cases} \frac{2}{\alpha}\mathrm{i}^n \mathrm{e}^{-\mathrm{i}n\theta_{\mathrm{inc}}}\mathrm{e}^{\mathrm{i}\alpha X}, & \text{for} \quad X > 0, \\ \frac{2}{\alpha}(-\mathrm{i})^n \mathrm{e}^{\mathrm{i}n\theta_{\mathrm{inc}}}\mathrm{e}^{-\mathrm{i}\alpha X}, & \text{for} \quad X < 0, \end{cases} \tag{SM1.4}$$

which for $L_{n-m}(X_2 - X_1)$ in (SM1.2) we have that $X_2 - X_1 < 0$.

For the remaining integral in (SM1.2) we use Green's second identity for $K_p \neq 1$ (having $K_p = 1$ leads to divergent integrals), for details see [SM1, Section B.], which

---

*Submitted to the editors October 2018.

**Funding:** This work was funded EPSRC (EP/M026205/1,EP/L018039/1) and support from the Isaac Newton Institute (EP/K032208/1).

† Department of Mechanical Engineering, The University of Sheffield, UK (arturgower@gmail.com, http://arturgower.github.io).

‡ School of Mathematics, University of Manchester, Oxford Road, Manchester M13 9PL, UK.

§ Isaac Newton Institute for Mathematical Sciences, 20 Clarkson Road, Cambridge CB3 0EH, UK

leads to

$$\int_{\substack{x_2>0 \\ \|\mathbf{x}_1-\mathbf{x}_2\|>a_{21}}} \mathcal{A}_n(kx_2)\mathrm{e}^{\mathrm{i}k(y_2-y_1)\sin\theta_{\mathrm{inc}}} F_{n-m}(k\mathbf{x}_1 - k\mathbf{x}_2)d\boldsymbol{x}_2 \\ = \frac{\mathrm{i}^m}{k^2}\left[\sum_{p=1}^{P} \mathrm{e}^{-\mathrm{i}m\varphi_p}\mathrm{e}^{\mathrm{i}K_p X_1\cos\varphi_p}\mathcal{B}^p_{nm} + \frac{\mathrm{e}^{\mathrm{i}X_1\cos\theta_{\mathrm{inc}}}}{\cos\theta_{\mathrm{inc}}}\mathrm{e}^{\mathrm{i}(n-m)\theta_{\mathrm{inc}}}\mathcal{C}_n\right], \tag{SM1.5}$$

where

$$\mathcal{B}^p_{nm} = A^p_n \frac{2\pi}{1-K_p^2}\mathcal{N}_{n-m}(K_p), \tag{SM1.6}$$

$$\mathcal{C}_n = 2(-\mathrm{i})^n \int_0^{\bar{X}} \mathcal{A}_n(X_2)\mathrm{e}^{-\mathrm{i}X_2\cos\theta_{\mathrm{inc}}}dX_2 \\ + 2\sum_{p=1}^{P}\mathrm{i}A^p_n\mathrm{e}^{-\mathrm{i}n\varphi_p}\frac{\mathrm{e}^{\mathrm{i}(K_p\cos\varphi_p-\cos\theta_{\mathrm{inc}})\bar{X}}}{K_p\cos\varphi_p-\cos\theta_{\mathrm{inc}}}. \tag{SM1.7}$$

where $\mathcal{N}_n(K) = \gamma R_o(H'_n(\gamma R_o)J_n(K\gamma R_o) - KH_n(\gamma R_o)J'_n(K\gamma R_o))$.

Substituting the above into (2.20), assuming $X_1 > \bar{X} + \gamma R_o$, we arrive at

$$\sum_{p=1}^{P}\mathrm{e}^{\mathrm{i}K_pX_1\cos\varphi_p}\mathrm{e}^{-\mathrm{i}m\varphi_p}\mathrm{i}^m\left[-k^2A^p_m + \mathfrak{n}\sum_{n=-\infty}^{\infty}T_m\mathcal{B}^p_{nm}\right] \\ + \frac{\mathrm{e}^{\mathrm{i}X_1\cos\theta_{\mathrm{inc}}}}{\cos\theta_{\mathrm{inc}}}\mathrm{i}^mT_m\left[\mathfrak{n}\sum_{n=-\infty}^{\infty}\mathrm{e}^{\mathrm{i}(n-m)\theta_{\mathrm{inc}}}\mathcal{C}_n + \mathrm{e}^{-\mathrm{i}m\theta_{\mathrm{inc}}}k^2\cos\theta_{\mathrm{inc}}\right] = 0. \tag{SM1.8}$$

As the above has to hold for every $X_1 > \bar{X} + \gamma R_o$ we conclude that the terms in the brackets have to be zero, which leads to equations (3.9) and (3.10).

**SM2. Complex least squares with a constraint.** Here we briefly show how to solve a least squares problem with a constraint. This is used in the paper to match the sum of effective waves (3.8) with the discrete form $\mathcal{A}^j_n$, while also satisfying the extinction equation (5.6), see Figure 3 for an illustration. The result in the paper is equation (5.11).

The variables we use below are not always directly related to variables that appear in the paper.

Assume the scalars $Y_i$ and vectors $\mathbf{X}_i$ are given, and we want to determine the unknown vector $\boldsymbol{\alpha}$ by matching $Y_i$ to $\boldsymbol{\alpha}^{\mathrm{T}}\mathbf{X}_i$ for every $i$, while also satisfying the scalar constraint (the extinction equation (5.6)) $\boldsymbol{w}^{\mathrm{T}}\boldsymbol{\alpha} = \mathbf{G}^{\mathrm{T}}\mathbf{Y} + c$. In the paper $i$ would represent the double index $j$ and $n$, with $j = L, \ldots, J$. To achieve this we minimise the difference:

$$\frac{1}{J-L}\min_{\boldsymbol{\alpha}}\sum_{j=L}^{J}|Y^j - \boldsymbol{\alpha}^{\mathrm{T}}\mathbf{X}^j|^2 \quad \text{subject to} \quad \mathbf{w}^{\mathrm{T}}\boldsymbol{\alpha} = \mathbf{G}^{\mathrm{T}}\mathbf{Y} + c. \tag{SM2.1}$$

The solution to the above is

$$\boldsymbol{\alpha} = \mathbf{Z}^{\mathrm{T}}\mathbf{Y} + \lambda\mathbf{V}^{-1}\overline{\mathbf{w}}, \tag{SM2.2}$$

where the over line $\overline{\mathbf{w}}$ denotes the conjugate of $\mathbf{w}$, and the matrices $\mathbf{V}$ and $\mathbf{Z}$ are such that

$$\mathbf{V} = \sum_i \overline{\mathbf{X}}_i (\mathbf{X}_i)^{\mathrm{T}}, \quad \mathbf{Z}^{\mathrm{T}}\mathbf{Y} = \sum_i \mathbf{V}^{-1}\overline{\mathbf{X}}_i Y_i, \tag{SM2.3}$$

so that

$$\mathbf{Z}^{\mathrm{T}} = [\cdots, \mathbf{V}^{-1}\overline{\mathbf{X}}_1, \mathbf{V}^{-1}\overline{\mathbf{X}}_2, \cdots]. \tag{SM2.4}$$

The Lagrangian multiplier $\lambda$ is determined by substituting (SM2.2) into the constraint in (SM2.1), which results in

$$\lambda w = \mathbf{G}^{\mathrm{T}}\mathbf{Y} + c - \mathbf{w}^T\mathbf{Z}^{\mathrm{T}}\mathbf{Y} \quad \text{with} \quad w = \mathbf{w}^T\mathbf{V}^{-1}\overline{\mathbf{w}}. \tag{SM2.5}$$

Substituting the above value for $\lambda$ into (SM2.2) we find that

$$\boldsymbol{\alpha} = \mathbf{L}^{\mathrm{T}}\mathbf{Y} + c w^{-1}\mathbf{V}^{-1}\overline{\mathbf{w}}, \tag{SM2.6}$$

with

$$\mathbf{L}^{\mathrm{T}} = \mathbf{Z}^{\mathrm{T}} + w^{-1}\mathbf{V}^{-1}\overline{\mathbf{w}}(\mathbf{G}^{\mathrm{T}} - \mathbf{w}^{\mathrm{T}}\mathbf{Z}^{\mathrm{T}}). \tag{SM2.7}$$

## SM3. The matching method.

The matching method can be summarised by Algorithm SM3.1. In detail: step 1 defines a tolerance *tol* for the field $\mathcal{A}_n(X)$ in the sense of the $\|\cdot\|_\infty$ norm. In step 2, the $P$ effective wavenumbers $K_p$ are found by searching initially from the initial guess $K_p = 0$, then increasing Im $K_p$ and searching for roots of $(3.9)_2$ until $P$ roots are found. In steps 4, we assume that the trapezoidal method was used to approximate the integrals in $X$, and we choose $h$ so that the expected error of the trapezoidal method is equal to the tolerance *tol*. In step 6, we choose $L$ so that the contribution of $p = P$ to (3.8) is less than *tol* at the depth $X = X^L$; that is, we want $|\mathrm{e}^{iX^L K_P \cos\varphi_P}| < tol$. This implies that the wavenumbers with even greater attenuation, which are not included in $\{K_1, \ldots, K_P\}$, would have no contribution to the field $\mathcal{A}_n(X)$ for $X > X^L$. In step 7, we choose $J$ to avoid the possibility of overfitting in the matching region $[X^L, X^J]$. At this point, if $L$ and $J$ are too large, we could go back and increase $P$, which would lead to $K_P$ having a large imaginary part, and therefore $L$ and $J$ would be smaller. Step 11 is a convergence check: as the matching method does not allow overfitting, the effective waves (3.8) and the discrete values $\mathcal{A}_n^j$ only match when both have converged. The final steps calculate the matched field $\mathcal{A}_n^M(X)$ (6.3).

REFERENCES

[SM1] A. L. Gower, M. J. A. Smith, W. J. Parnell, and I. D. Abrahams, *Reflection from a multi-species material and its transmitted effective wavenumber*, Proc. R. Soc. A, 474 (2018), p. 20170864, https://doi.org/10.1098/rspa.2017.0864.

[SM2] C. M. Linton and P. A. Martin, *Multiple scattering by random configurations of circular cylinders: Second-order corrections for the effective wavenumber*, The Journal of the Acoustical Society of America, 117 (2005), p. 3413, https://doi.org/10.1121/1.1904270.

[SM3] P. A. Martin, *Multiple scattering by random configurations of circular cylinders: Reflection, transmission, and effective interface conditions*, The Journal of the Acoustical Society of America, 129 (2011), pp. 1685–1695, https://doi.org/10.1121/1.3546098.

**Algorithm SM3.1** Matching method

1: Let $tol$ be the tolerance for the field $\mathcal{A}_n(X)$ (6.3).
2: Calculate $K_p$ $(3.9)_2$ for the first $P$ with the smallest positive $\mathrm{Im}\, K_p$.
3: Calculate $\varphi_p$ and $a_n^p$ (3.2,$3.9_1$,3.11).
4: Let $h = (12tol/|\mathcal{A}_0''(0)|)^{1/3}$ when setting $A_0^p = 1$ in (3.8).
5: Let $K_P$ have the largest imaginery part out of $\{K_1, \ldots, K_P\}$.
6: Let $L = -\mathrm{round}(\log(tol)/(h\mathrm{Im}\, K_P \cos\varphi_P))$.
7: Let $J = L + \max\{L, \lceil 1.5P \rceil\}$.
8: Let $X^j = jh$ for $j = 0, 1, \ldots, J$.
9: Calculate $\mathbb{E}$, $\mathbb{R}$, $\mathbb{M}$, $\mathbb{B}$, and $\mathbb{L}$ (5.2,5.4,5.12, 5.16).
10: Solve (5.14) for $\mathbb{A}$.
11: **if** the sum $(5.10)_1$ is too large **then**
12: decrease $tol$, increase $P$, and return to step 2.
13: **else**
14: calculate $\mathcal{A}_n(X)$ from (6.3).
15: **end if**
16: **return** $\mathcal{A}_n^M(X) = \mathcal{A}_n(X)$
